# Supplementary material for: Vapor-liquid equilibrium of water with the MB-pol many-body potential
Source: arXiv:2103.06978 ancillary file (2021-04-28)
Supplement: Supplementary file 1 [file si.pdf]

# Supplementary Material for:
# Vapor-liquid equilibrium of water with the MB-pol many-body potential

Maria Carolina Muniz,[1, a)] Thomas E. Gartner III,[2, a)] Marc Riera,[3] Christopher Knight,[4] Shuwen Yue,[1] Francesco Paesani,[3, 5, 6, b)] and Athanassios Z. Panagiotopoulos[1, c)]

[1)] *Department of Chemical and Biological Engineering, Princeton University, Princeton, New Jersey 08544, USA*
[2)] *Department of Chemistry, Princeton University, Princeton, New Jersey 08544, USA*
[3)] *Department of Chemistry and Biochemistry, University of California, San Diego, La Jolla, California 92093, USA*
[4)] *Computational Science Division, Argonne National Laboratory, Argonne, Illinois 60439, USA*
[5)] *Materials Science and Engineering, University of California San Diego, La Jolla, California 92093, USA*
[6)] *San Diego Supercomputer Center, University of California San Diego, La Jolla, California 92093, USA*

(Dated: 28 April 2021)

## I. LIQUID STRUCTURE

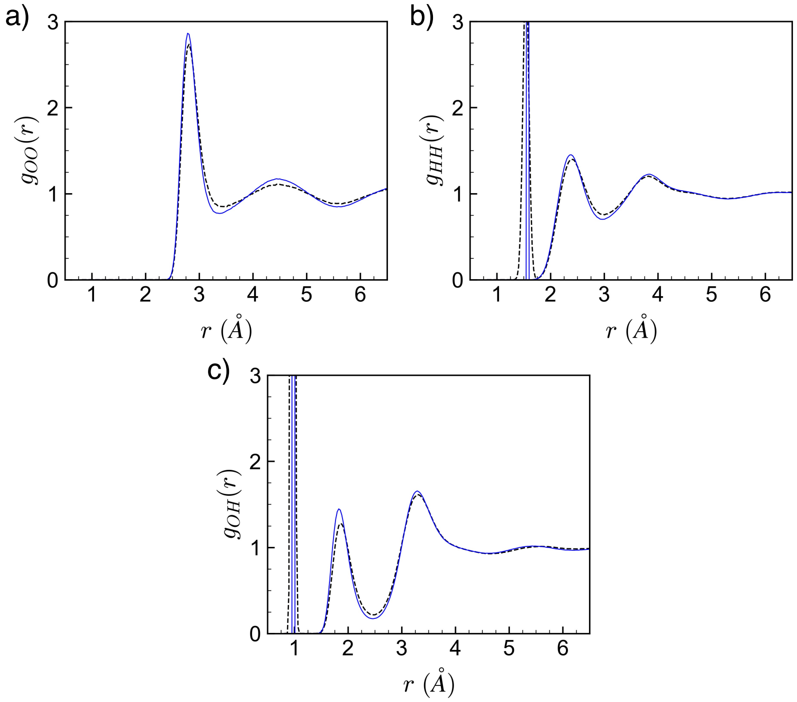


FIG. 1. (a.) Oxygen-oxygen, (b.) hydrogen-hydrogen, and (c.) oxygen-hydrogen radial distribution functions $g(r)$ for a 512-molecule isothermal-isobaric MB-pol simulation at $T = 298$ K and $P = 1$ atm. Black dashed lines are the standard (flexible) MB-pol model and blue solid lines are the rigid variant with bonds and angles constrained to the average values from the flexible simulation.

[a)] These authors contributed equally to this work.
[b)] Electronic mail: fpaesani@ucsd.edu
[c)] Electronic mail: azp@princeton.edu

## II. SURFACE TENSION

TABLE I. Surface tension results (N/m). Uncertainties indicate 95% confidence intervals that were obtained from dividing simulations into 10 blocks.

| T(K) | Exp[1]. | Flexible-512 | Rigid-512 | Rigid-1024 |
|---|---|---|---|---|
| 400 | 0.054 | 0.053 ± 0.005 | 0.053 ± 0.001 | 0.053 ± 0.002 |
| 425 | 0.048 | 0.046± 0.003 | 0.047 ± 0.002 | 0.047 ± 0.002 |
| 450 | 0.043 | 0.047 ± 0.003 | 0.041 ± 0.001 | 0.042 ± 0.003 |
| 475 | 0.037 | 0.036 ± 0.004 | 0.035 ± 0.002 | 0.037 ± 0.003 |
| 500 | 0.031 | 0.028 ± 0.004 | 0.032 ± 0.001 | 0.029 ± 0.001 |
| 525 | 0.026 | 0.025± 0.003 | 0.025 ± 0.002 | 0.022 ± 0.002 |
| 550 | 0.020 | 0.021 ± 0.004 | 0.020 ± 0.002 | 0.018 ± 0.002 |
| 575 | 0.014 | 0.013 ± 0.003 | 0.015 ± 0.002 | 0.009 ± 0.003 |
| 600 | 0.008 | – | – | 0.007 ± 0.002 |

## III. VAPOR PRESSURES

TABLE II. Vapor pressure results (MPa). Uncertainties indicate 95% confidence intervals that were obtained from dividing simulations into 10 blocks.

| T(K) | Exp.[1] | Flexible-512 | Rigid-512 | Rigid-1024 |
|---|---|---|---|---|
| 400 | 0.24577 | 0.34 ± 0.01 | 0.298 ± 0.002 | 0.270 ± 0.001 |
| 425 | 0.50025 | 0.56 ± 0.02 | 0.592 ± 0.004 | 0.524 ± 0.006 |
| 450 | 0.93220 | 0.98 ± 0.03 | 1.06 ± 0.01 | 0.854 ± 0.006 |
| 475 | 1.6160 | 1.8 ± 0.1 | 1.72 ± 0.01 | 1.78 ± 0.02 |
| 500 | 2.6392 | 2.7 ± 0.1 | 2.82 ± 0.02 | 2.99 ± 0.02 |
| 525 | 4.1019 | 4.6 ± 0.2 | 5.44 ± 0.05 | 4.53 ± 0.04 |
| 550 | 6.1172 | 9.2 ± 0.4 | 6.91 ± 0.06 | 7.05 ± 0.06 |
| 575 | 8.8140 | 9.4 ± 0.4 | 10.4 ± 0.1 | 10.7 ± 0.1 |
| 600 | 12.345 | – | – | 14.5 ± 0.2 |

## IV. ENTHALPY OF VAPORIZATION

TABLE III. Enthalpy of vaporization results (kJ/mol). Uncertainties indicate 95% confidence intervals that were obtained from dividing simulations into 10 blocks.

| T(K) | Exp.[1] | Flexible-512 | Rigid-512 | Rigid-1024 |
|---|---|---|---|---|
| 400 | 39.3227 | 39 ± 1 | 39.4 ± 0.8 | 39.8 ± 0.5 |
| 425 | 37.975 | 38 ± 1 | 37.8 ± 0.7 | 38.0 ± 0.7 |
| 450 | 36.486 | 37 ± 1 | 36.5 ± 0.5 | 36.7 ± 0.5 |
| 475 | 34.814 | 34 ± 1 | 34.8 ± 0.3 | 34.9 ± 0.3 |
| 500 | 32.914 | 32 ± 1 | 32.6 ± 0.3 | 32.5 ±0.2 |
| 525 | 30.725 | 30 ± 1 | 28.9 ± 0.8 | 30.0 ± 0.4 |
| 550 | 28.155 | 25 ± 1 | 27.1 ± 0.3 | 26.9 ± 0.3 |
| 575 | 25.052 | 23 ± 1 | 23.2 ± 0.3 | 22.5 ± 0.4 |
| 600 | 21.123 | – | – | 18.6 ± 0.3 |

## V. COEXISTENCE DENSITIES

TABLE IV. Liquid (L) and vapor (V) coexistence densities (g/cm$^3$). Uncertainties indicate 95% confidence intervals that were obtained from dividing simulations into 10 blocks.

| T(K) | Phase | Exp[1]. | Flexible-512 | Rigid-512 | Rigid-1024 |
|---|---|---|---|---|---|
| 400 | L | 0.93749 | 0.934± 0.001 | 0.9273± 0.0002 | 0.9284 ± 0.0006 |
| 400 | V | 0.0013694 | 0.0019± 0.0006 | 0.0017± 0.0003 | 0.0015 ± 0.0002 |
| 425 | L | 0.91527 | 0.910± 0.001 | 0.9025± 0.0005 | 0.9041 ± 0.0005 |
| 425 | V | 0.0026693 | 0.0029 ± 0.0006 | 0.0032 ± 0.0004 | 0.0028 ± 0.0003 |
| 450 | L | 0.89034 | 0.883± 0.002 | 0.8761±0.0003 | 0.8773 ± 0.0006 |
| 450 | V | 0.0048120 | 0.005± 0.001 | 0.0055± 0.0005 | 0.0044 ± 0.0004 |
| 475 | L | 0.86249 | 0.854± 0.002 | 0.8463± 0.0006 | 0.8470 ± 0.0005 |
| 475 | V | 0.0081598 | 0.0095± 0.0009 | 0.0086 ± 0.0004 | 0.0090 ± 0.0004 |
| 500 | L | 0.83131 | 0.821±0.002 | 0.8114 ±0.0007 | 0.8138 ± 0.0009 |
| 500 | V | 0.013199 | 0.0147±0.0009 | 0.0141 ±0.0007 | 0.0152 ± 0.0007 |
| 525 | L | 0.79613 | 0.783±0.003 | 0.769 ±0.007 | 0.775 ± 0.001 |
| 525 | V | 0.020617 | 0.023± 0.002 | 0.030 ± 0.006 | 0.023 ± 0.002 |
| 550 | L | 0.75581 | 0.73±0.01 | 0.730 ±0.001 | 0.731 ± 0.001 |
| 550 | V | 0.031474 | 0.05± 0.02 | 0.037 ±0.002 | 0.0379 ± 0.0021 |
| 575 | L | 0.70830 | 0.687±0.005 | 0.677 ±0.003 | 0.674 ± 0.007 |
| 575 | V | 0.047607 | 0.057±0.006 | 0.061 ±0.003 | 0.065 ± 0.006 |
| 600 | L | 0.64941 | – | – | 0.61 ± 0.01 |
| 600 | V | 0.072842 | – | – | 0.095 ± 0.008 |

## VI. REFERENCES

[1] P. Linstrom and W. Mallard, *NIST Chemistry WebBook, NIST Standard Reference Database Number 69* (National Institute of Standards and Technology, Gaithersburg MD) p. 20899.
